# Supplementary material for: Toward a Secure Crowdsourced Location Tracking System
Source: arXiv:2106.00217 source file (2021-06-01)
Supplement: Supplementary file 1 [file appendix.tex]

\appendix

% \begin{figure}[t]
%     \centering
%     \includegraphics[width=\columnwidth]{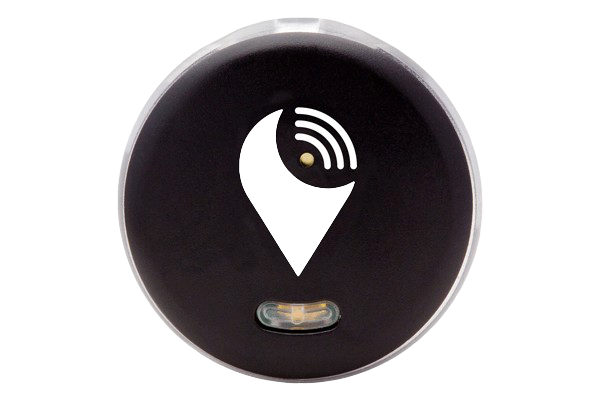}
%     \caption{Example \ac{TD}: TrackR Pixel }
%     \label{fig:trackr-pixel}
% \end{figure}

\section{Crowdsourced Tracking Systems}
\label{app:tracking_systems_details}

\tbl{tbl:crowdcommts} shows the messages sent from the~\acp{TApp} to the corresponding~\acp{TS}, along with the contacted REST endpoints.

\begin{table*}[]
\centering
\tiny
%\scriptsize
\caption{Communication mechanism used by various tracking services with the corresponding~\ac{TS}. The payload column indicates the relevant data used in each of the corresponding request. We use N/A to indicate that the payload is not relevant.}
\label{tbl:crowdcommts}
\vspace{-0.3cm}
\begin{tabular}{|c|c|c|c|c|c|c|}
\hline
\multirow{3}{*}{\textbf{Tracking System}} & \multicolumn{6}{c|}{\textbf{Communication with TS}}                                                                                        \\ \cline{2-7} 
                                          & \multicolumn{2}{c|}{\textbf{Owner Registration}} & \multicolumn{2}{c|}{\textbf{Location Update}} & \multicolumn{2}{c|}{\textbf{Location Query}} \\ \cline{2-7} 
                                          & \textbf{End Point}    & \textbf{Payload}    & \textbf{End Point}     & \textbf{Payload}     & \textbf{End Point}     & \textbf{Payload}    \\ \hline
TrackR                                    & \begin{tabular}[c]{@{}c@{}}\texttt{POST }\url{https://platform.thetrackr.com/rest}\\ \url{/item?usertoken=[USERTOKEN]}\end{tabular}                  & \texttt{trackerid} &\begin{tabular}[c]{@{}c@{}}\texttt{PUT }\url{https://platform.thetrackr.com/rest}\\ \url{/tracker/batch/secure/[DEVICETOKEN]}\end{tabular}   & \begin{tabular}[c]{@{}c@{}}\texttt{trackerid}, \\Location coordinates\end{tabular}            & \begin{tabular}[c]{@{}c@{}}\texttt{GET }\url{https://platform.thetrackr.com/rest}\\ \url{/item?usertoken=[USERTOKEN]}\end{tabular}                   &     N/A         \\ \hline
CUBE                                      & \begin{tabular}[c]{@{}c@{}}\texttt{POST }\url{https://net.cubetracker.com/}\\ \url{api/devices?}\\ \url{AddCubeWithMac=[MACADDRESS]&}\\ \url{type=CUBE&hardware=[HARDWARETYPE]}\end{tabular}                  & Bluetooth MAC address & \begin{tabular}[c]{@{}c@{}}\texttt{PUT }\url{https://net.cubetracker.com/}\\ \url{api/devices}\end{tabular}                   & \begin{tabular}[c]{@{}c@{}} Bluetooth MAC address,\\Location coordinates \end{tabular}             & \begin{tabular}[c]{@{}c@{}}\texttt{GET }\url{https://net.cubetracker.com/}\\ \url{api/devices?emailID=[EMAILID]}\end{tabular}                   & N/A             \\ \hline
Chipolo                                   & \begin{tabular}[c]{@{}c@{}}\texttt{GET }\url{https://api.chipolo.net/v2/}\\ \url{user/[USERID]/lookup/mac/[MAC ADDRESS]} \\ \\ \texttt{POST }\url{https://api.chipolo.net/v2/}\\ \url{user/[USERID]/chipolo}\end{tabular}                  & \begin{tabular}[c]{@{}c@{}}GET Request Returns:\\ \texttt{chipoloid} \\ \\ POST Request Payload:\\ \texttt{chipoloid}\end{tabular}       & \begin{tabular}[c]{@{}c@{}}\texttt{GET }\url{https://api.chipolo.net/v2/}\\ \url{user/[USERID]/device/[DEVICEID]} \\ \\ \texttt{POST }\url{https://api.chipolo.net/v2/}\\ \url{user/[DEVICEID]/chipolo/[chipoloid]}\end{tabular}                   & \begin{tabular}[c]{@{}c@{}} GET Request Returns:\\ \texttt{chipoloid} \\ \\ POST Request Payload:\\ \texttt{chipoloid}\\ Location coordinates\end{tabular}            & \begin{tabular}[c]{@{}c@{}}\texttt{GET }\url{https://api.chipolo.net/v2/}\\ \url{user/[USERID]/state}\end{tabular}                   & N/A \\ \hline
Pebblebee                                 & \begin{tabular}[c]{@{}c@{}}\texttt{POST }\url{https://api.pebblebee.com/v1/}\\ \url{devices/[MAC ADDRESS]}\end{tabular}                  & N/A  & \begin{tabular}[c]{@{}c@{}}\texttt{POST }\url{https://data.pebblebee.com/v1/}\\ \url{devices/data/batch}\end{tabular}                   & \begin{tabular}[c]{@{}c@{}} Bluetooth MAC address,\\Location coordinates \end{tabular}            & \begin{tabular}[c]{@{}c@{}}\texttt{GET }\url{https://api.pebblebee.com/v1/}\\ \url{devices/[MAC ADDRESS]}\end{tabular}                   & N/A             \\ \hline
Tile                                 & \begin{tabular}[c]{@{}c@{}}\texttt{POST }\url{https://production.tile-api.com/api/v1/}\end{tabular}                  & Encrypted  & \begin{tabular}[c]{@{}c@{}}\texttt{POST }\url{https://production.tile-api.com/api/v1/}\end{tabular}                   & Encrypted            & \begin{tabular}[c]{@{}c@{}}\texttt{GET }\url{https://production.tile-api.com/api/v1/}\end{tabular}                   & N/A             \\ \hline
\end{tabular}
\end{table*}
